# Supplementary material for: Snakes in the Plane: Controllable Gliders in a Nanomagnetic Metamaterial
Source: arXiv:2505.01116 ancillary file (2025-05-02)
Supplement: Supplementary file 1 [file supplementary.pdf]

# Supplementary information: Snakes in the Plane: Controllable Gliders in a Nanomagnetic Metamaterial

Arthur Penty<sup>1\*</sup>, Johannes H. Jensen<sup>1</sup>, Ida Breivik<sup>2</sup>,  
Anders Strømberg<sup>2</sup>, Erik Folven<sup>2</sup>, Gunnar Tufte<sup>1</sup>

<sup>1</sup>Department of Computer Science, Norwegian University of Science and  
Technology, Trondheim, Norway.

<sup>2</sup>Department of Electronic Systems, Norwegian University of Science  
and Technology.

\*Corresponding author(s). E-mail(s): [arthur.penty@ntnu.no](mailto:arthur.penty@ntnu.no);

## 1 Supplementary Discussion

### 1.1 MuMax3 simulations

To assess the viability of experimental realisations, the snake was first verified in micro-magnetic simulations using MuMax3 [1]. Fig. 1 shows snapshots from the MuMax3 simulations, where a leftwards snake is successfully realised. As can be seen, a  $10 \times 10$  pinwheel ASI is first initialised with a snake in the centre, as shown in Fig. 1 (0). Then the  $bBaA$  clock protocol is applied, for two clock cycles, as shown in Fig. 1 (1-8), using  $H^+ = 34$  mT and  $H^- = 33$  mT. The strength of each clock field was increased from zero to the target field strength using a ramp function  $\tanh(15ft)$  with  $f = 10^8$ . The ramp function results in an initially rapid increase of the field strength, followed by a slow approach towards the target field strength for a duration of 10 ns. Ramp duration was found to be sufficient to allow the nanomagnets' internal spin wave dynamics to settle between each field application. The simulated nanomagnets are stadium-shaped with dimensions  $220 \text{ nm} \times 80 \text{ nm} \times 10 \text{ nm}$ , arranged with a lattice spacing of 280 nm. Simulation parameters include saturation magnetisation  $M_S = 860 \text{ kA m}^{-1}$ , exchange stiffness  $A_{\text{ex}} = 1.3 \times 10^{-11} \text{ J m}^{-1}$ , damping constant  $\alpha = 0.01$ , a world size of  $1024 \times 1024$  cells and a cell size of  $5 \text{ nm} \times 5 \text{ nm} \times 10 \text{ nm}$ .

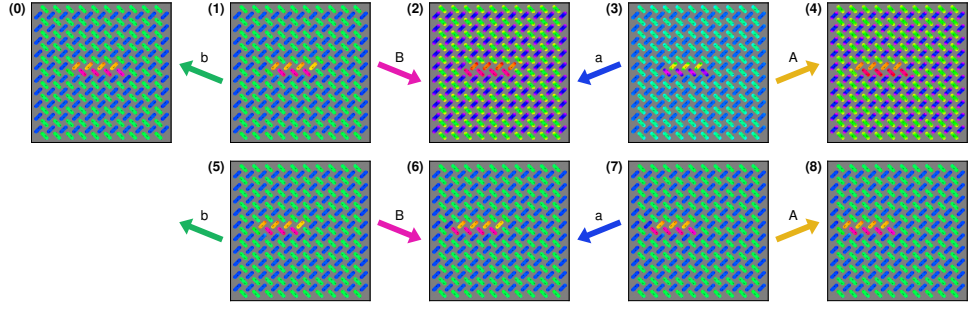

**Fig. 1:** MuMax3 simulations of a snake in  $10 \times 10$  pinwheel ASI. (0) shows the initial state of the snake. (1-8) shows the state of the snake during  $bBaA$  clocking. The field arrow to the left of each snapshot indicate the clock field which precedes it. A video of the simulation is provided in Supplementary Movie 3.

## 1.2 Experimental realisation of clocking with equal strength clock fields

To experimentally verify that  $H^-$  must be strictly less than  $H^+$ , we polarise and write a new initial snake state, as shown in Fig. 2 (0). We then find  $H^+$  by applying the  $B$  clock field with increasing field strength, until the snake grows, as shown in Fig. 2 (1). The  $B$  field is used to find  $H^+$  because, in this particular written initial state, the next unlocked nanomagnet at the head of the snake is in sublattice  $L_b$ . When we apply the next clock field,  $a$ , with  $H^- = H^+ = 21$  mT, almost the entire snake state disappears, as shown in Fig. 2 (2). To verify that this effect is not due to variations in the switching fields of the nanomagnets, we repeat this process for two more snakes in different parts of the array.

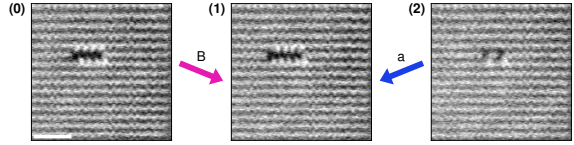

**Fig. 2:** Experimental clocking of a snake with  $H^- = H^+$ . MFM-micrographs of part of a  $100 \times 100$  pinwheel ASI. (0) shows the initial state of the snake.  $H^+$  is found by applying the  $B$  field with increasing field strength until the snake grows (1). In (2), the  $a$  field is applied with  $H^- = H^+ = 21$  mT, resulting in most of the nanomagnets in the snake switching, making the snake state disappear.

## 2 Supplementary Figures

### 2.1 Leftwards and rightwards moving snakes

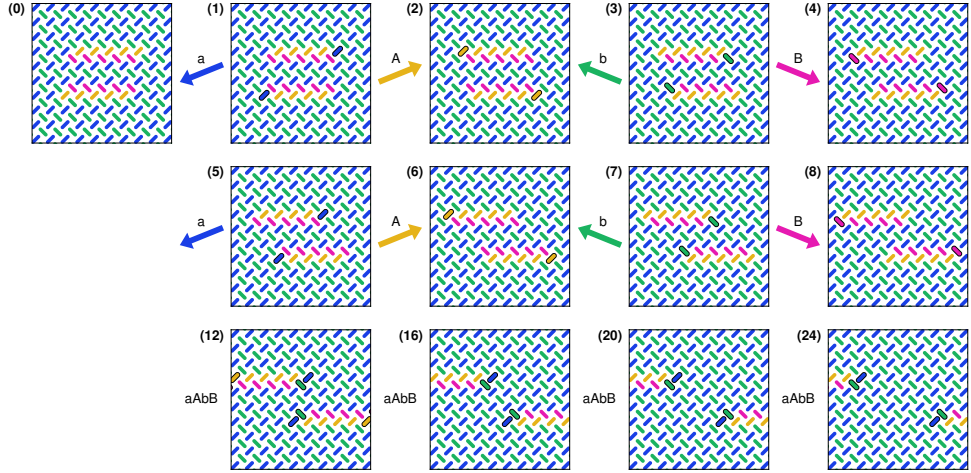

**Fig. 3:** Leftwards and rightwards moving snake gliders in pinwheel ASI. Each snapshot shows a zoomed-in view of a  $50 \times 50$  system, at different points during the  $aAbB$  clock protocol. (0) shows the initial state of the snakes, two elongated orange/pink domains in the centre of a blue/green background domain. (1-8) shows the state of the snakes during  $aAbB$  clocking, where magnets that change state between snapshots are highlighted by a solid black outline. The field arrow to the left of each snapshot indicates the clock field which precedes it. The top snake moves leftwards, while the bottom snake moves rightwards, through alternate shrinking ( $a$  and  $b$ ) and growing ( $A$  and  $B$ ) steps. The bottom row continues the series, showing only snapshots after a complete clock cycle (four clock fields are applied between each snapshot). A video of the simulation is provided in Supplementary Movie 2.

## 2.2 Neighbour influence analysis for all fields

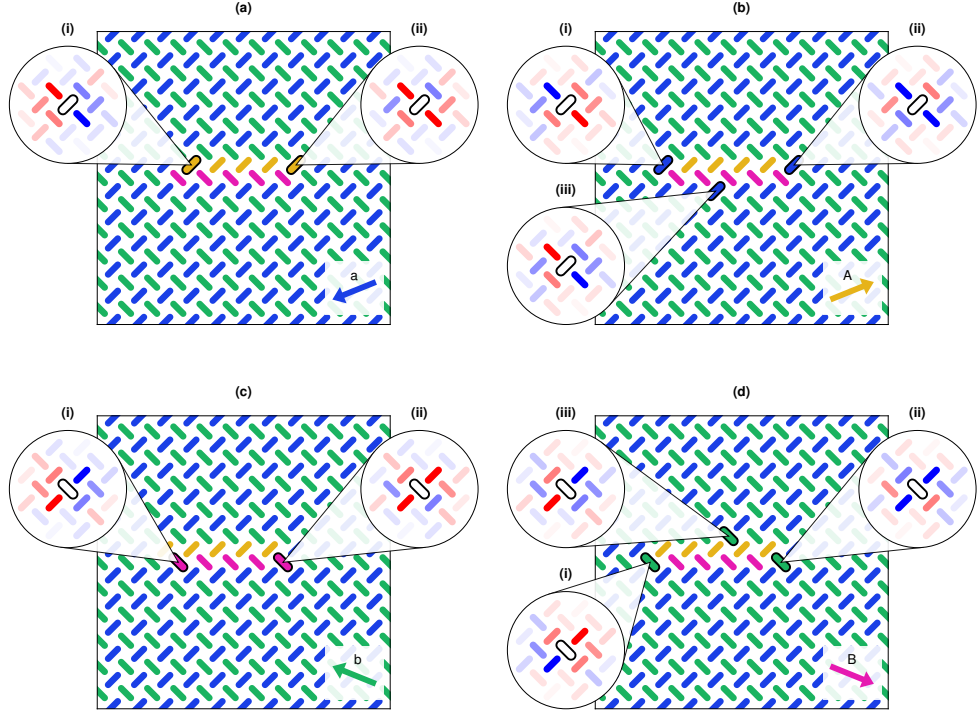

**Fig. 4:** Neighbour influence during (a) shrinking of  $L_a$ , (b) growth of  $L_a$ , (c) shrinking of  $L_b$  and (d) growth of  $L_b$ . The insets depict the switching influence from the neighbours of the highlighted magnet. Stronger red signifies that the magnet is biasing the highlighted magnet towards switching, and stronger blue signifies that the magnet is biasing the highlighted magnet away from switching. Notice how the switching influences for (c) are mirror images of (a), and similarly for (d) and (b).

## References

- [1] Vansteenkiste, A., Leliaert, J., Dvornik, M., Helsen, M., Garcia-Sanchez, F., Van Waeyenberge, B.: The design and verification of MuMax3. AIP Advances 4(10), 107133 (2014) <https://doi.org/10.1063/1.4899186>
